# Supplementary material for: CPS++: Improving Class-level 6D Pose and Shape Estimation From Monocular Images With Self-Supervised Learning
Source: arXiv:2003.05848 source file (2020-09-11)
Supplement: Supplementary file 1 [file 7_supplement.tex]

\section{Detailed Results}

In Table~\ref{tab:pose_cps} and Table~\ref{tab:pose_cpspp} we present individual graphs for each evaluated metric. For rotation and translation, we measure the angular deviation and euclidean distance between the ground truth and the prediction. 3D IoU calculates the intersection over union between the estimated and ground truth 3D bounding box. Average Distance of Predicted Point Sets (APP) applies the Average Distance of Indistinguishable Model Points (ADI) in both directions (see paper and supplementary video for more details). For each metric we report the mean Average Precision for different thresholds. 

\section{Additional qualitative results on the synthetic validation and real test dataset.}

In Fig.~\ref{fig:pose_cps_synthetic}, we show more qualitative results for the synthetic NOCS validation dataset. From left to right: We show the regressed 6D poses and 3D scales. We also render an orthogonal projection on the XZ and XY plane, similar as in the paper.
We employ these projections to demonstrate that we can compute accurate 6D poses and 3D scales without being prone to ambiguities (scale~\vs~depth) due to monocular data. Finally, we illustrate one exemplary regressed shape for each image to show that we can accurately estimate the perceived objects' 3D meshes.

In Fig.~\ref{fig:qual_test}, we show more qualitative results for the real NOCS test data. On the left, we render the regressed 6D pose and 3D scale, constituted as 3D bounding box, onto the input image. We thereby illustrate the prediction and ground truth in \emph{green} and \emph{red}, respectively. In the middle, we also overlay the regressed shapes onto the input image to show that they fit to the perceived objects. On the right, we depict the same scene from a different viewpoint, in order to demonstrate that the poses and scales are also metrically correct. 

\begin{table*}[t]
    \centering

    \includegraphics[width=0.24\linewidth,trim={0 0 1.6cm 1cm},clip]{figs/supplement/aps/cps/IoU_3D_AP_0.0-1.0.png}
    \includegraphics[width=0.24\linewidth,trim={0 0 1.6cm 1cm},clip]{figs/supplement/aps/cps/Pose_Only_mAP_0-15degree.png}
    \includegraphics[width=0.24\linewidth,trim={0 0 1.6cm 1cm},clip]{figs/supplement/aps/cps/Pose_Only_mAP_0-15cm.png} 
    \includegraphics[width=0.24\linewidth,trim={0 0 1.6cm 1cm},clip]{figs/supplement/aps/cps/APP_AP_0.0-1.0.png}\\
    \includegraphics[width=0.24\linewidth,trim={0 0 1.6cm 1cm},clip]{figs/supplement/aps/cpsicp/IoU_3D_AP_0.0-1.0.png}
    \includegraphics[width=0.24\linewidth,trim={0 0 1.6cm 1cm},clip]{figs/supplement/aps/cpsicp/Pose_Only_mAP_0-15degree.png}
    \includegraphics[width=0.24\linewidth,trim={0 0 1.6cm 1cm},clip]{figs/supplement/aps/cpsicp/Pose_Only_mAP_0-15cm.png} 
    \includegraphics[width=0.24\linewidth,trim={0 0 1.6cm 1cm},clip]{figs/supplement/aps/cpsicp/APP_AP_0.0-1.0.png}\\
    \scalebox{1}{
        \begin{tabular}{|c||c|c|c|}
        \bottomrule
        $\cps$ & 3D IOU @ (0.25 / 0.5) & 10\degree \& 10cm & 3D APP @ (0.2 / 0.5) \\
             \Xhline{1pt}
            Bottle & 31.3 / 8.3 & 28.0 & 16.6 / 56.6 \\
            Bowl & 24.6 / 3.4 & 44.5 & 13.5 / 46.8 \\
            Camera & 20.7 / 5.4 & 7.2 & 16.2 / 40.4 \\
            Can & 17.9 / 6.0 & 77.9 & 11.2 / 33.7 \\ 
            Laptop & 62.8 / 22.2 & 15.7 & 44.1 / 85.1 \\
            Mug & 16.4 / 4.1 & 16.7 & 12.8 / 35.1 \\
            \toprule
        \end{tabular}
    }%ktion AP: 87.085091 83.797050 75.036331
    \\
    %\vspace*{3mm}
    \scalebox{1}{
        \begin{tabular}{|c||c|c|c|}
        \bottomrule
        $\cps$ w ICP & 3D IOU @ (0.25 / 0.5) &  5\degree \& 5cm  / 10\degree \& 10cm  & 3D APP @ (0.2 / 0.5) \\
             \Xhline{1pt}
            Bottle & 83.9 / 78.9 & 86.5 / 95.2 & 79.4 / 84.78 \\
            Bowl & 95.7 / 87.5 & 22.4 / 54.4 & 94.6 / 95.9 \\
            Camera & 91.8 / 41.9 & 10.0 / 35.1 & 92.4 / 94.3 \\
            Can & 91.8 / 84.6 & 94.6 / 96.7 & 90.6 / 93.0 \\ 
            Laptop & 96.8 / 87.8 & 36.4 / 71.3 & 95.9 / 98.5 \\
            Mug & 81.2 / 41.9 & 7.1 / 30.3 & 81.1 / 81.5 \\
            \toprule
        \end{tabular}
    }%ktion AP: 87.085091 83.797050 75.036331
    %\vspace*{3mm}
    \caption{Detailed results for each object with and without ICP on the synthetic validation dataset from (Wang et al., 2019). Top: We plot AP scores for 3D IoU, rotation and translation, and APP with respect to increasing thresholds. Bottom: We report AP scores for 3D IoU, rotation and translation, and APP at commonly employed thresholds}%\vspace{-2em}}
    \label{tab:pose_cps}
\end{table*}

\begin{table*}[t]
    \centering
    \includegraphics[width=0.24\linewidth,trim={0 0 1.6cm 1cm},clip]{figs/supplement/aps/cpspp/IoU_3D_AP_0.0-1.0.png}
    \includegraphics[width=0.24\linewidth,trim={0 0 1.6cm 1cm},clip]{figs/supplement/aps/cpspp/Pose_Only_mAP_0-15degree.png}
    \includegraphics[width=0.24\linewidth,trim={0 0 1.6cm 1cm},clip]{figs/supplement/aps/cpspp/Pose_Only_mAP_0-15cm.png} 
    \includegraphics[width=0.24\linewidth,trim={0 0 1.6cm 1cm},clip]{figs/supplement/aps/cpspp/APP_AP_0.0-1.0.png}\\
    \includegraphics[width=0.24\linewidth,trim={0 0 1.6cm 1cm},clip]{figs/supplement/aps/cpsppicp/IoU_3D_AP_0.0-1.0.png}
    \includegraphics[width=0.24\linewidth,trim={0 0 1.6cm 1cm},clip]{figs/supplement/aps/cpsppicp/Pose_Only_mAP_0-15degree.png}
    \includegraphics[width=0.24\linewidth,trim={0 0 1.6cm 1cm},clip]{figs/supplement/aps/cpsppicp/Pose_Only_mAP_0-15cm.png} 
    \includegraphics[width=0.24\linewidth,trim={0 0 1.6cm 1cm},clip]{figs/supplement/aps/cpsppicp/APP_AP_0.0-1.0.png}\\
    
    \scalebox{1}{
        \begin{tabular}{|c||c|c|c|}
        \bottomrule
        $\cps$++ & 3D IOU @ (0.25 / 0.5) & 10\degree \& 10cm & 3D APP @ (0.2 / 0.5) \\
             \Xhline{1pt}
            Bottle & 21.7 / 5.2 & 28.9 & 15.9 / 42.8 \\
            Bowl & 73.9 / 22.1 & 49.6 & 48.2 / 96.6 \\
            Camera & 49.6 / 10.5 & 5.7 & 41.2 / 70.4 \\
            Can & 29.4 / 6.6 & 9.9 & 12.7 / 46.4 \\
            Laptop & 99.0 / 54.8 & 18.6 & 86.7 / 99.9 \\
            Mug & 52.4 / 7.1 & 2.2 & 41.3 / 85.7 \\
            \toprule
        \end{tabular}
    }%ktion AP: 87.085091 83.797050 75.036331
    %\vspace*{3mm}
    \\
     \scalebox{1}{
        \begin{tabular}{|c||c|c|c|}
        \bottomrule
        $\cps$++ w ICP & 3D IOU @ (0.25 / 0.5) &  5\degree \& 5cm  / 10\degree \& 10cm  & 3D APP @ (0.2 / 0.5) \\
             \Xhline{1pt}
             Bottle & 58.2 / 45.2 & 43.1 / 74.6 & 52.5 / 60.9 \\
             Bowl & 99.8 / 99.8 & 35.6 / 92.7 & 99.8 / 99.8 \\
             Camera & 89.8 / 57.2 & 0.2 / 3.5 & 89.3 / 90.0 \\
             Can & 62.7 / 56.1 & 60.9 / 85.2 & 48.0 / 66.2 \\
             Laptop & 89.8 / 57.2 & 5.6 / 54.4 & 99.5 / 100.0 \\
             Mug & 97.3 / 86.5 & 6.0 / 41.3 & 97.1 / 97.4 \\
         \toprule
        \end{tabular}
    }%ktion AP: 87.085091 83.797050 75.036331
    \caption{Detailed results for each object  with and without ICP on the real test dataset from (Wang et al., 2019). Top: We plot AP scores for 3D IoU, rotation and translation, and APP with respect to increasing thresholds. Bottom: We report AP scores for 3D IoU, rotation and translation, and APP at commonly employed thresholds}%\vspace{-2em}}
    \label{tab:pose_cpspp}
\end{table*}

\begin{figure*}[t]
    \centering
    \begin{tabular}{cccc}
        3D Bounding Box &  XZ-plane Projection &  XY-plane Projection& Recovered Mesh \\ 
        \includegraphics[width=0.22\textwidth]{figs/supplement/qualitative/synthetic/cps_1_3d} &
        \includegraphics[width=0.22\textwidth]{figs/supplement/qualitative/synthetic/cps_1_bev} &
        \includegraphics[width=0.22\textwidth]{figs/supplement/qualitative/synthetic/cps_1_bev_front} &  
        \includegraphics[height=82pt, width=84pt]{figs/supplement/qualitative/synthetic/cps_1_mesh}  \\
        \includegraphics[width=0.22\textwidth]{figs/supplement/qualitative/synthetic/cps_2_3d} &
        \includegraphics[width=0.22\textwidth]{figs/supplement/qualitative/synthetic/cps_2_bev} &
        \includegraphics[width=0.22\textwidth]{figs/supplement/qualitative/synthetic/cps_2_bev_front} &  
        \includegraphics[height=82pt, width=84pt]{figs/supplement/qualitative/synthetic/cps_2_mesh}  \\
        \includegraphics[width=0.22\textwidth]{figs/supplement/qualitative/synthetic/cps_3_3d} &
        \includegraphics[width=0.22\textwidth]{figs/supplement/qualitative/synthetic/cps_3_bev} &
        \includegraphics[width=0.22\textwidth]{figs/supplement/qualitative/synthetic/cps_3_bev_front} &  
        \includegraphics[height=82pt, width=84pt]{figs/supplement/qualitative/synthetic/cps_3_mesh}  \\
        \includegraphics[width=0.22\textwidth]{figs/supplement/qualitative/synthetic/cps_4_3d} &
        \includegraphics[width=0.22\textwidth]{figs/supplement/qualitative/synthetic/cps_4_bev} &
        \includegraphics[width=0.22\textwidth]{figs/supplement/qualitative/synthetic/cps_4_bev_front} &  
        \includegraphics[height=82pt, width=84pt]{figs/supplement/qualitative/synthetic/cps_4_mesh}  \\
        \includegraphics[width=0.22\textwidth]{figs/supplement/qualitative/synthetic/cps_5_3d} &
        \includegraphics[width=0.22\textwidth]{figs/supplement/qualitative/synthetic/cps_5_bev} &
        \includegraphics[width=0.22\textwidth]{figs/supplement/qualitative/synthetic/cps_5_bev_front} &  
        \includegraphics[height=82pt, width=84pt]{figs/supplement/qualitative/synthetic/cps_5_mesh}  \\
        \includegraphics[width=0.22\textwidth]{figs/supplement/qualitative/synthetic/cps_6_3d} &
        \includegraphics[width=0.22\textwidth]{figs/supplement/qualitative/synthetic/cps_6_bev} &
        \includegraphics[width=0.22\textwidth]{figs/supplement/qualitative/synthetic/cps_6_bev_front} &  
        \includegraphics[height=82pt, width=84pt]{figs/supplement/qualitative/synthetic/cps_6_mesh}  \\
    \end{tabular}
    \caption{\textbf{Qualitative results on synthetic validation dataset.} Left: Exemplary object pose estimations with rendered 3D bounding boxes, coordinate systems and shape meshes, overlaid on top of the respective input images. Centre: BEV images emphasizing accurate depth estimation of multiple objects in the scene (Our results are visualized in \emph{green} and ground truth in \emph{red}.). Right: Exemplary 3D mesh for each image, rendered with Meshlab (Cignoni et al., 2008)}
    \label{fig:pose_cps_synthetic}
\end{figure*}

\begin{figure*}[t!]
    \centering
    \includegraphics[width=0.95\linewidth]{figs/supplement/qualitative/test/cps_3.jpg}\\
    \includegraphics[width=0.95\linewidth]{figs/supplement/qualitative/test/cps_4.jpg}\\
    \includegraphics[width=0.95\linewidth]{figs/supplement/qualitative/test/cps_5.jpg}
    \includegraphics[width=0.95\linewidth]{figs/supplement/qualitative/test/cps_6.jpg}\\
    \includegraphics[width=0.95\linewidth]{figs/supplement/qualitative/test/cps_7.jpg}\\
\end{figure*}

\begin{figure*}[t!]
    \centering
    \includegraphics[width=0.95\linewidth]{figs/supplement/qualitative/test/cps_8.jpg}\\
     
    \caption{\textbf{Qualitative results on real test dataset.} Left: Object pose estimations with rendered 3D bounding boxes, coordinate systems (Centre:) and shape mesh, overlaid on top of the respective real input images. Right: We show an alternative viewpoint to the right to avoid ambiguities through projection.}
    \label{fig:qual_test}
\end{figure*}
